# Supplementary material for: Learning Unified Distance Metric Across Diverse Data Distributions with Parameter-Efficient Transfer Learning
Source: arXiv:2309.08944 source file (2025-01-19)
Supplement: Supplementary file 1 [file lora_ablation.tex]

\begin{table*}[!h]
\setlength{\tabcolsep}{2pt}
\fontsize{7.5}{9}\selectfont
\centering
\begin{tabularx}{1.0\textwidth}
    {
      p{0.19\textwidth}
      >{\centering\arraybackslash}p{0.12\textwidth}
      >{\centering\arraybackslash}p{0.058\textwidth}
      >{\centering\arraybackslash}p{0.058\textwidth}
      >{\centering\arraybackslash}p{0.058\textwidth}
      >{\centering\arraybackslash}p{0.058\textwidth}
      >{\centering\arraybackslash}p{0.058\textwidth}
      >{\centering\arraybackslash}p{0.058\textwidth}
      >{\centering\arraybackslash}p{0.058\textwidth}
      >{\centering\arraybackslash}p{0.058\textwidth}
      >{\centering\arraybackslash}p{0.058\textwidth}
      >{\centering\arraybackslash}p{0.058\textwidth}
      >{\centering\arraybackslash}X
      >{\centering\arraybackslash}X
      }
    \toprule
    \multicolumn{1}{l}{\multirow{2}{*}[-3.5mm]{Methods}}&
    \multicolumn{1}{c}{\textbf{Params~(M)}} &
    \multicolumn{8}{c}{\textbf{Dataset-specific Accuracy}} & \multicolumn{2}{c}{\textbf{Universal Accuracy}} \\ 
    \cmidrule(lr){2-2}  \cmidrule(lr){3-10}  
    \cmidrule(lr){11-12} & 
    \multicolumn{1}{c}{Train~/~Total} &
    CUB & Cars & SOP & In\text{-}Shop & NABirds & Dogs & Flowers & Aircraft & Unified & Harmonic \\ \midrule
\multicolumn{1}{l}{LoRA} & 2.4 / 24.1 & 77.0 & 70.9 & 81.3 & 86.2 & 70.8 & 79.1 & 98.9 & 59.7 & 76.1 & 76.5 \\
\multicolumn{1}{l}{Stochastic LoRA} & 2.4 / 24.1 & 83.0 & 71.7 & 80.0 & 83.4 & 78.0 & \textbf{84.7} & \textbf{99.4} & 64.3 & 77.3 & 79.4 \\
\multicolumn{1}{l}{PUMA + LoRA} & 4.8 / 26.5 & 76.8 & 77.6 & 83.9 & 90.4 & 72.2 & 79.5 & 98.9& 65.0 & 78.7 & 79.3 \\
\multicolumn{1}{l}{PUMA + Stochastic LoRA} & 4.8 / 26.5 &83.1 & 83.8 & \textbf{84.7} & \textbf{91.2} & \textbf{83.9} & 73.5 & 99.2 & 72.2 & \textbf{81.5} & 83.9 \\ \midrule
\multicolumn{1}{l}{\ccol PUMA} & \ccol 2.5 / 24.2 & \ccol \textbf{83.9} & {\ccol \textbf{84.3}}&  {\ccol {84.0}} & {\ccol 89.8} & {\ccol {79.2}} & {\ccol 84.1} & { \ccol{99.3}} &  \ccol \textbf{72.6} &{ \ccol{81.3}}& \ccol\textbf{84.1} \\
\bottomrule
\end{tabularx}
\caption{Performance comparison of LoRA~\cite{hu2021lora} variants and their combination with PUMA. The bottleneck dimension of LoRA is set to 128, the same as that of the Adapter. The keep probability for the stochastic version of LoRA is set to $p=0.5$.}
\label{subtab:lora_ablation}
\end{table*}
