# Supplementary material for: Learning Unified Distance Metric Across Diverse Data Distributions with Parameter-Efficient Transfer Learning
Source: arXiv:2309.08944 source file (2025-01-19)
Supplement: Supplementary file 2 [file loss_ablation.tex]

\begin{table*}[!h]
\setlength{\tabcolsep}{2pt}
\fontsize{7.5}{9}\selectfont
\centering
\begin{tabularx}{1.0\textwidth}
    {
      p{0.03\textwidth}
      >{\centering\arraybackslash}X
      >{\centering\arraybackslash}X
      >{\centering\arraybackslash}X
      >{\centering\arraybackslash}X
      >{\centering\arraybackslash}X
      >{\centering\arraybackslash}X
      >{\centering\arraybackslash}X
      >{\centering\arraybackslash}X
      >{\centering\arraybackslash}X
      >{\centering\arraybackslash}X
      >{\centering\arraybackslash}X
      >{\centering\arraybackslash}X}
     \toprule

    \multicolumn{1}{l}{\multirow{2}{*}[-3.5mm]{Methods}}&
    \multicolumn{8}{c}{\textbf{Dataset-specific Accuracy}} & \multicolumn{2}{c}{\textbf{Universal Accuracy}} \\ \cmidrule(lr){2-9}  
    \cmidrule(lr){10-11} & 
    CUB & Cars & SOP & In\text{-}Shop & NABirds & Dogs & Flowers & Aircraft & Unified & Harmonic \\ \midrule
\multicolumn{1}{l}{Triplet} & 75.2 & 36.5 & 78.5 & 79.9 & 69.3 & 78.3 & 98.7 & 39.8 & 71.1 & 62.3 \\
\multicolumn{1}{l}{Margin} & 75.4 & 38.2 & 78.4 & 79.1 & 70.1 & 79.2 & 98.9 & 40.2 & 71.3 & 63.1 \\
\multicolumn{1}{l}{MS} & 72.5 & 30.8 & 80.5 & 86.1 & 66.1 & 74.9 & 98.6 & 37.2 & 71.1 & 58.9 \\
\multicolumn{1}{l}{SupCon} & 42.5 & 12.4 & 50.0 & 55.6 & 33.2 & 46.3 & 86.2 & 20.0 & 39.0 & 31.3 \\
\multicolumn{1}{l}{PA} & 82.1 & 54.8 & 83.2 & 89.6 & 77.7 & 83.4 & \textbf{99.4} & 56.1 & 77.8 & 75.2 \\
\multicolumn{1}{l}{ProxyNCA++} & 49.6 & 19.1 & 62.3 & 62.3 & 39.7 & 61.3 & 93.9 & 27.1 & 52.8 & 41.3 \\
\multicolumn{1}{l}{SoftTriple} & 82.7 & 81.2 & 79.9 & 85.6 & 78.6 & \textbf{84.5} & 99.3 & 69.7 & 78.5 & 82.0 \\
\multicolumn{1}{l}{CosFace} & 83.8 & 80.9 & 82.5 & 89.3 & 78.7 & 83.8 & 99.3 & 69.0 & 80.0 & 82.6 \\
\multicolumn{1}{l}{ArcFace} & 82.3 & 43.6 & 80.8 & 85.9 & 77.3 & 84.0 & 99.3 & 44.9 & 75.3 & 68.8 \\
\multicolumn{1}{c}{\ccol CurricularFace} & \ccol \textbf{83.9} & \multicolumn{1}{c}{\ccol \textbf{84.3}}&  \multicolumn{1}{c}{\ccol \textbf{84.0}} & \multicolumn{1}{c}{\ccol \textbf{89.8}} & \multicolumn{1}{c}{\ccol \textbf{79.2}} & \multicolumn{1}{c}{\ccol 84.1} & \multicolumn{1}{c}{ \ccol{99.3}} &  \multicolumn{1}{c}{\ccol \textbf{72.6}} &\multicolumn{1}{c}{ \ccol\textbf{81.3}}&  \ccol \textbf{84.1} \\
\bottomrule
\end{tabularx}
\caption{Recall@1 of PUMA using different loss functions. Note that our default metric learning objective is CurriculumFace loss~\cite{huang2020curricularface}.}
\label{subtab:loss_ablation}
\end{table*}
