# Supplementary material for: Learning Unified Distance Metric Across Diverse Data Distributions with Parameter-Efficient Transfer Learning
Source: arXiv:2309.08944 source file (2025-01-19)
Supplement: Supplementary file 3 [file map_rp.tex]

\begin{table*}[!t]

\fontsize{7.5}{9.5}\selectfont
\centering
\begin{tabularx}{1.0\textwidth}
    {
      p{0.1\textwidth}
      >{\centering\arraybackslash}X
      >{\centering\arraybackslash}X
      >{\centering\arraybackslash}X
      >{\centering\arraybackslash}X
      >{\centering\arraybackslash}X
      >{\centering\arraybackslash}X
      >{\centering\arraybackslash}X
      >{\centering\arraybackslash}X
      >{\centering\arraybackslash}X
      >{\centering\arraybackslash}X
      >{\centering\arraybackslash}X
      >{\centering\arraybackslash}X
      >{\centering\arraybackslash}X
      >{\centering\arraybackslash}X
      >{\centering\arraybackslash}X
      >{\centering\arraybackslash}X
      >{\centering\arraybackslash}X
      >{\centering\arraybackslash}X
      }
     \toprule
    \multicolumn{1}{l}{\multirow{2}{*}[-3.5mm]{Methods}} & \multicolumn{2}{c}{CUB} & \multicolumn{2}{c}{Cars} & \multicolumn{2}{c}{SOP} & \multicolumn{2}{c}{InShop} & \multicolumn{2}{c}{NABirds} & \multicolumn{2}{c}{Dogs} & \multicolumn{2}{c}{Flowers} & \multicolumn{2}{c}{Aircraft} & \multicolumn{2}{c}{Harmonic} \\ \cmidrule(lr){2-3} \cmidrule(lr){4-5} \cmidrule(lr){6-7} \cmidrule(lr){8-9} \cmidrule(lr){10-11} \cmidrule(lr){12-13} \cmidrule(lr){14-15} \cmidrule(lr){16-17} \cmidrule(lr){18-19}
    & M@R & RP & M@R & RP & M@R & RP & M@R & RP & M@R & RP & M@R & RP & M@R & RP & M@R & RP & M@R & RP \\     
    \midrule

    \multicolumn{19}{l}{(a) \textit{\textbf{Dataset-specific models with ViT Backbone}}} \\ \midrule
     PA & 46.2 & 55.5 & 27.8 & 38.3 & \textbf{51.5} & \textbf{54.2} &{65.5} & {68.1} &37.0 & 47.1&48.5&58.8  &91.7 &\textbf{93.3} &21.4 &\textbf{34.7} &40.5 & 51.6\\ 
     CosFace & 43.4 & 53.8 & 26.4 & 36.8& 49.6 & 52.5&63.6 & 66.3&35.9 & 46.1&47.3 &57.7&\textbf{92.1} &93.0 &20.1 &32.8 &38.8&49.9\\ 
     CurricularFace & 43.8 & 53.5& 24.0& 34.8& 48.9 & 52.2 &62.0 & 65.3 &36.4 &46.8&48.4 &58.8&91.1 &93.0&17.9 &31.3 & 37.0 & 49.1   \\ \midrule
      \multicolumn{19}{l}{(b) \textit{\textbf{Universal models by full fine-tuning}}} \\ \midrule
     PA & 41.9 &51.5& 22.9 &34.1& 50.7 &53.7&\textbf{67.7} &\textbf{70.3}&33.0 &43.4&39.5 &51.0&70.3 &74.0&18.5 &31.8& 35.4& 47.3 \\
     CosFace & 36.6 & 46.7 & 21.3 & 32.1& 48.4 & 51.4 &64.1 & 66.8& 28.7& 39.2&30.4 &42.7&85.1 &87.0 &17.3 &30.1 &32.3 &44.3\\ 
    CurricularFace &40.8 &50.7&22.3 &33.4&47.6 &50.8&62.8 &65.7&31.6 &42.6&38.3 &50.2&87.2 &88.8& 17.6 &30.5 &34.3&46.5 \\
    \ccol Ours & \ccol \textbf{48.5} &\ccol \textbf{57.5}&\ccol \textbf{28.1} &\ccol \textbf{38.5}&\ccol 50.3 &\ccol 53.3&\ccol 65.2 &\ccol 68.0&\ccol \textbf{38.8} &\ccol \textbf{49.1}&\ccol \textbf{48.7} &\ccol \textbf{59.0}&\ccol 91.4 &\ccol 92.5&\ccol \textbf{21.8}&\ccol 34.4&\ccol \textbf{41.1}&\ccol \textbf{52.0} \\
\bottomrule 
\end{tabularx}
\caption{
Mean Average Precision at R (M@R) and R-Precision (RP) of metric learning baselines and ours with the eight datasets.}
\label{subtab:comparison_maprp}
\end{table*}
