# Supplementary material for: Learning Unified Distance Metric Across Diverse Data Distributions with Parameter-Efficient Transfer Learning
Source: arXiv:2309.08944 source file (2025-01-19)
Supplement: Supplementary file 4 [file recall_k.tex]

\begin{table*}[!t]

\fontsize{6}{8}\selectfont
\setlength{\tabcolsep}{1pt}
\centering
\begin{tabularx}{1.0\textwidth}
    {
      m{0.09\textwidth}
      >{\centering\arraybackslash}X
      >{\centering\arraybackslash}X
      >{\centering\arraybackslash}X
      >{\centering\arraybackslash}X
      >{\centering\arraybackslash}X
      >{\centering\arraybackslash}X
      >{\centering\arraybackslash}X
      >{\centering\arraybackslash}X
      >{\centering\arraybackslash}X
      >{\centering\arraybackslash}X
      >{\centering\arraybackslash}X
      >{\centering\arraybackslash}X
      >{\centering\arraybackslash}X
      >{\centering\arraybackslash}X
      >{\centering\arraybackslash}X
      >{\centering\arraybackslash}X
      >{\centering\arraybackslash}X
      >{\centering\arraybackslash}X
      >{\centering\arraybackslash}X
      >{\centering\arraybackslash}X
      >{\centering\arraybackslash}X
      >{\centering\arraybackslash}X
      >{\centering\arraybackslash}X
      >{\centering\arraybackslash}X
      }
     \toprule
    \multicolumn{1}{l}{\multirow{2}{*}[-3.5mm]{Methods}} & \multicolumn{3}{c}{CUB} & \multicolumn{3}{c}{Cars} & \multicolumn{3}{c}{SOP} & \multicolumn{3}{c}{InShop} & \multicolumn{3}{c}{NABirds} & \multicolumn{3}{c}{Dogs} & \multicolumn{3}{c}{Flowers} & \multicolumn{3}{c}{Aircraft}  \\ \cmidrule(lr){2-4} \cmidrule(lr){5-7} \cmidrule(lr){8-10} \cmidrule(lr){11-13} \cmidrule(lr){14-16} \cmidrule(lr){17-19} \cmidrule(lr){20-22} \cmidrule(lr){23-25}
    & R@1 & R@2 & R@4 & R@1 & R@2 & R@4& R@1 & R@10 & R@10$^2$ & R@1 & R@10 & R@20& R@1 & R@2 & R@4& R@1 & R@2 & R@4& R@1 & R@2 & R@4 & R@1 & R@2 & R@4 \\     
    \midrule

    \multicolumn{25}{l}{\fontsize{6.5}{9}\selectfont{ (a) \textit{\textbf{{Dataset-specific models by full fine-tuning}}}}} \\ \midrule

    Triplet  & 81.1 & 88.1& 92.9&  75.2 & 84.2& 90.2&  80.2 & 84.9& 88.6&  87.4 & 92.1& 95.2& 75.2 &83.4 &89.5 &  81.0& 88.4& 93.3&  99.1 & 99.5& 99.7&  64.7 & 76.6 & 86.6\\
     Margin  & 79.4 & 87.8& 92.3&  78.0 & 86.0 & 91.9 &  79.8 & 84.6& 88.5&  86.0& 91.6& 94.9&  74.6 & 83.1& 89.4&  80.3 & 87.8& 92.7&  99.0 & 99.5& 99.7& 66.8 & 79.0 & 87.1\\
     MS  & 80.0 & 87.0& 91.8&  83.7 & 90.3& 94.1&  81.4 & 85.5& 89.0&  90.8 & 93.7& 95.9&  68.1&77.4 &84.3 &  75.8 & 83.8& 89.6&  97.4 & 98.4& 98.8&  64.7 & 77.6 & 86.3\\
     PA & 80.2 & 87.8 & 92.4&  83.7 & 90.2&94.6 &  84.4 & 88.2& 91.1&  91.5 & 94.5& 96.7&  69.6 & 78.4& 85.5&  84.2 & 91.1& 94.7&  99.0 & 99.4& 99.6&  67.9 & 78.1 & 87.1  \\
     % PNCA++  & 72.3 & 81.4& 87.7&  55.1 & 66.6& 76.7&  63.8 & 69.7& 75.1&  74.6 & 90.5& 85.6&  51.4 & 61.7& 71.0&  65.6 & 75.4 & 83.1&  94.3 & 95.9& 96.9&  54.0 & 68.1 & 79.0  \\
     SoftTriple  & 80.5 & 88.0 & 92.0&  80.0 & 88.2 & 93.2&  82.9 & 86.8& 90.0&  88.7 & 92.7&95.5 &  75.9 & 84.0& 89.9&  82.1 & 89.3& 94.0& 99.4& 99.7& 99.8&  65.4 & 77.3 & 86.7 \\
     CosFace  & 78.8 & 86.6 & 91.5&  83.2 & 89.5 & 93.9 & 83.2 & 87.1& 90.1&  89.6 & 93.4 & 95.7& 71.4 & 80.4& 87.0&  79.2 & 87.1& 92.3&  99.2 &99.6 & 99.7 &  61.4 &  74.3 & 83.7 \\
     ArcFace  & 76.8 & 85.1 & 90.9&  79.4 & 86.5 & 91.6  & 83.4 & 87.3& 90.1&  90.3 & 93.7 &96.2 &  61.0 &70.8 &79.1 &  76.1 & 84.2& 90.2&  99.2 & 99.6& 99.7&  60.0 & 74.1 & 84.7 \\
     CurricularFace & 79.7 & 87.9& 92.4&  81.3 & 88.7 & 93.6  & 83.2 & 87.3& 90.4&  88.2 & 92.7& 95.4&  75.3 & 84.0& 89.7&  81.2 & 88.9& 93.9&  99.1 & 99.6& 99.8&  63.9 &76.5 & 85.6\\
     Hyp &78.8 & 87.1 & 92.3& 78.2 & 85.6 & 91.0 & 83.6  & 88.0 & 91.1& 91.5 & 95.2 &97.1 &  71.0 & 79.7& 86.4&  72.6 & 82.0& 89.1&  98.7 & 99.3& 99.5& 65.7 & 78.2 & 86.7 \\ \midrule
     
    \multicolumn{25}{l}{\fontsize{6.5}{9}\selectfont{ (b) \textit{\textbf{{Universal models by full fine-tuning}}}}} \\ \midrule

     Triplet  &74.5 & 83.6 & 90.6 &  35.4 & 47.7& 60.5&  80.2 & 92.3& 97.3&  85.7 & 97.1& 98.1&  68.2 & 78.4& 86.0&  77.1 & 87.1& 92.4&  98.7 & 99.4 & 99.8 & 40.9 & 52.2 & 64.2 \\
     Margin  & 72.5 & 83.1& 90.5&  36.7& 47.8& 59.8&  80.0 & 92.1& 97.3&  84.1 & 96.8& 97.9&  67.4 & 77.8& 85.5&  74.8 & 84.9& 91.5&  98.5 & 99.2&99.5 &  40.4 &51.4 & 62.7 \\
     MS  & 66.3 & 77.1 & 85.0 &  22.9 &32.6 & 44.7&  78.9 & 90.9 & 96.7&  87.2& 96.0& 87.2&  58.6& 69.4& 78.5&  69.8 & 80.4& 88.0&  97.3 & 98.4& 98.8& 31.5 & 42.7 & 54.5 \\
     PA  & 77.2 & 85.4&90.5 &  73.1 & 82.1& 88.5&  83.7 & 93.5& 97.3&  {91.9} & 98.1& 98.7&  71.5& 80.2& 86.8&  78.1 & 86.3& 91.4&  96.4 & 97.3& 97.0&  62.7 & 74.9 & 84.4 \\
     % PNCA++ & 59.2 & 71.4& 81.4&  21.6 & 30.8& 41.5&  53.8 & 74.1& 88.4&  57.9 & 82.5& 87.5&  49.8 & 61.8& 72.3&  65.4 & 77.3& 86.0&  93.8 & 96.5& 97.8&  33.8 & 44.5 & 55.9  \\
     SoftTriple & 78.9 & 87.0& 91.7&  77.0 & 85.8& 91.6&  81.3 & 92.1& 86.6&  88.6 & 97.4& 98.2&  73.8 & 82.8& 89.2&  79.3 & 87.6& 92.5&  99.1 & 99.5& 99.8&  64.4 & 77.6 & 86.1\\
     CosFace  & 74.2 & 83.4& 89.2&  73.5 & 82.5& 88.7&  82.5 & 92.4&96.4 &  90.0 & 97.4& 98.3&  69.7 & 78.9& 85.9&  74.1 & 83.8& 89.8&  98.7 &99.2 &99.5 & 59.7 & 72.1 & 81.8 \\
     ArcFace  & 70.8 & 80.0 & 86.3&  25.9 & 36.7& 49.3&  63.9 & 72.8& 79.0&  58.9 & 74.7& 77.8&  64.0 & 72.8& 79.9&  70.3 & 79.0& 85.9&  97.2 & 98.5& 99.1&  31.7 & 43.4 & 56.1 \\
     CurricularFace  & 78.3 & 87.0& 91.7&  77.9 & 86.4& 92.1&  82.0 & 92.7& 96.9&  89.1 & 97.5& 98.5&  73.0 & 82.2& 88.7&  79.3 &87.7 & 92.9&  99.1 & 99.4& 99.6&  65.6 & 78.0 & 99.3 \\
     Hyp  & 79.2 & 87.8 & 92.7&  60.6 & 73.1 & 82.8&  83.5 & 93.9& 97.7&  90.9 &98.2 & 98.9&  73.6 & 82.6& 89.2&  81.9 & 89.5& 94.3&  99.1 & 99.5& 99.8&  56.3 & 69.0 & 79.9  \\
     Ours&  {83.9} & 90.2& 93.5&   {84.3}& 90.3& 94.3&   {84.0} & 93.7& 97.5&  89.8 & 98.0& 98.6&  {79.2} & 86.7& 91.9&   84.1 & 90.7& 94.5&  99.3 & 99.6&99.8 &   72.6 & 82.7 & 94.3 \\  
     % PA~\cite{kim2020proxy} &\multicolumn{1}{c}{512}  & 78.0 & & &  76.5 & & &  85.0 & & &  {92.2} & & &  72.8 & & &  79.2 & & &  96.7 & & &  67.0 \\
     % SoftTriple~\cite{Qian_2019_ICCV} &\multicolumn{1}{c}{512}  & 80.1 & & &  81.2 & & &  82.0 & & &  88.3 & & &  75.6 & & &  80.7 & & &  99.2 & & &  67.4  \\
     % CosFace~\cite{wang2018cosface} & \multicolumn{1}{c}{512}  &  74.7 & & &  77.7 & & &  83.8 & & &  90.5 & & &  71.0 & & &  75.4 & & &  99.0 & & &  63.4\\
     % ArcFace~\cite{deng2019arcface} &\multicolumn{1}{c}{512}  & 70.6 & & &  37.2 & & &  66.7 & & &  61.7 & & &  63.6 & & &  71.0 & & &  97.7 & & &  34.8 \\
     % CurricularFace~\cite{huang2020curricularface} & 512  & 80.5 & & &  80.8 & & &  83.2 & & &  89.6 & & &  75.5 & & &  80.8 & & &  99.2 & & &  68.7 \\
     % Hyp~\cite{ermolov2022hyperbolic} &\multicolumn{1}{c}{512}  & 80.5 & & &  65.7 & & &  84.1 & & &  91.2 & & &  75.6 & & &  82.3 & & &  99.1 & & &  57.6 \\
     % Ours& \multicolumn{1}{c}{ 512} &  {84.6} & & &   {85.7} & & &   {85.1} & & &  \multicolumn{1}{c}{ 90.9} & & &  \multicolumn{1}{c}{ {80.1}} & & &  \multicolumn{1}{c}{ {84.5}} & & &  \multicolumn{1}{c}{ {99.3}} & & &   \multicolumn{1}{c}{ {74.4}} \\  
\bottomrule 
\end{tabularx}
\caption{
Recall@$k$ (R@$k$) of metric learning baselines and ours with the eight datasets.}
\label{subtab:comparison_recallatk}
\end{table*}
