# Supplementary material for: Learning Unified Distance Metric Across Diverse Data Distributions with Parameter-Efficient Transfer Learning
Source: arXiv:2309.08944 source file (2025-01-19)
Supplement: Supplementary file 5 [file standard.tex]

\begin{table*}[!t]
\fontsize{8}{9.5}\selectfont
\centering
\setlength{\tabcolsep}{5.05pt}
\begin{tabularx}{1.0 \linewidth}
    {
      p{0.2\linewidth}
      >{\centering\arraybackslash}p{0.15\linewidth}
      >{\centering\arraybackslash}X
      >{\centering\arraybackslash}X
      >{\centering\arraybackslash}X
      >{\centering\arraybackslash}X
      >{\centering\arraybackslash}X
      >{\centering\arraybackslash}X
      >{\centering\arraybackslash}X
      }
     \toprule

    \multicolumn{1}{l}{\multirow{2}{*}[-3.5mm]{Methods}}&
    \multicolumn{1}{c}{\textbf{Params~(M)}} &
    \multicolumn{4}{c}{\textbf{Dataset-specific}} &  \multicolumn{2}{c}{\textbf{Universal}}\\
    \cmidrule(lr){2-2} \cmidrule(lr){3-6} \cmidrule(lr){7-8} &  \multicolumn{1}{c}{Train~/~Total} & CUB &  Cars &   SOP &  InShop & Unified &  Harmonic \\ \midrule

  \multicolumn{8}{l}{(a) \textit{\textbf{Dataset-specific models} with CNN Backbone}} \\ \midrule
     \multicolumn{1}{l}{Margin\textsuperscript{128}~\cite{sampling_matters}}  & 95.1~/~95.1 & 63.9 &79.6  &72.7 & - & - & -\\
    % NSoftmax\textsuperscript{128}~\cite{zhai2018classification} & 95.1~/~95.1 &56.5 &81.6 &75.2 & 86.6 & - & 73.0 \\
    MIC\textsuperscript{128}~\cite{roth2019mic} & 95.1~/~95.1  &66.1 & 82.6 &77.2 &88.2 & - & 77.6 \\
    MS\textsuperscript{512}~\cite{wang2019multi} & 47.3~/~47.3 &65.7 &84.1 &78.2 & 89.7 & - & 78.4 \\
    PA\textsuperscript{512}~\cite{kim2020proxy} & 47.3~/~47.3 &68.4  &86.1  &79.1  &91.5 & - & 79.2 \\
    NSoftmax\textsuperscript{512}~\cite{zhai2018classification} & 98.2~/~98.2 &61.3  &84.2 &78.2  &86.6 & - & 76.2 \\
    PNCA++\textsuperscript{512}~\cite{teh2020proxynca++} & 98.2~/~98.2 &69.0  &\textbf{86.5} &80.7 & 90.4 & - &80.7 \\ \midrule
\multicolumn{8}{l}{(b) \textit{\textbf{Dataset-specific models} with ViT Backbone}} \\ \midrule
     Triplet\textsuperscript{128}~\cite{Schroff2015} & \multicolumn{1}{c}{86.9~/~86.9} & 81.1 & 75.2 & 80.2 & 87.4 & 61.5 &80.7 \\
     Margin\textsuperscript{128}~\cite{sampling_matters}  & \multicolumn{1}{c}{86.9~/~86.9}& 79.4 & 78.0 & 79.8 & 86.0 & 66.0 &80.7 \\
     MS\textsuperscript{128}~\cite{wang2019multi}   & \multicolumn{1}{c}{86.9~/~86.9} & 80.0 & 83.7 & 81.4 & 90.8 & 65.3 &83.8 \\
     PA\textsuperscript{128}~\cite{kim2020proxy}  &\multicolumn{1}{c}{86.9~/~86.9} & 80.2 & 83.7 & 84.4 & 91.5 & 62.7 &84.8 \\
     SoftTriple\textsuperscript{128}~\cite{Qian_2019_ICCV}  &\multicolumn{1}{c}{86.9~/~86.9} & 80.5 & 80.0 & 82.9 & 88.7  & 68.4&82.9\\
     CosFace\textsuperscript{128}~\cite{wang2018cosface} & \multicolumn{1}{c}{86.9~/~86.9} & 78.8 & 83.2 & 83.2 & 89.6  & 67.2 &83.5 \\
     ArcFace\textsuperscript{128}~\cite{deng2019arcface}  & \multicolumn{1}{c}{86.9~/~86.9} & 76.8 & 79.4 & 83.4 & 90.3  & 67.1& 82.2 \\
     CurricularFace\textsuperscript{128}~\cite{huang2020curricularface} &\multicolumn{1}{c}{86.9~/~86.9} & 79.7 & 81.3 & 83.2 & 88.2 & 67.6& 83.0 \\
     Hyp\textsuperscript{128}~\cite{ermolov2022hyperbolic}  & \multicolumn{1}{c}{86.9~/~86.9} &78.8 & 78.2 & 83.6 & 91.5 & 28.3 &82.7\\ \midrule
    % \midrule
    \multicolumn{8}{l}{(c) \textit{\textbf{Universal Models} with ViT Backbone}} \\ \midrule
% \multicolumn{1}{l}{{ViT-S}$^{128}$} ㅣ
     Triplet\textsuperscript{128}~\cite{Schroff2015} &\multicolumn{1}{c}{21.7~/~21.7} & 69.5 & 35.6 & 79.8 & 85.9 & 76.0 & 60.0 \\
     Margin\textsuperscript{128}~\cite{sampling_matters} &\multicolumn{1}{c}{21.7~/~21.7} & 70.0 & 37.1 & 79.8 & 82.4 & 75.7 & 60.7 \\
     MS\textsuperscript{128}~\cite{wang2019multi} &\multicolumn{1}{c}{21.7~/~21.7} & 62.5 & 23.8 & 80.2 & 87.6 & 75.0 & 48.8 \\
     PA\textsuperscript{128}~\cite{kim2020proxy} &\multicolumn{1}{c}{21.7~/~21.7} &  75.4 & 72.6 & 84.0 & \textbf{91.7} & 83.6 & 80.2 \\
     SoftTriple\textsuperscript{128}~\cite{Qian_2019_ICCV} &\multicolumn{1}{c}{21.7~/~21.7} & 76.8 & 76.9 & 82.3 & 89.2 & 82.6 & 81.0 \\
     CosFace\textsuperscript{128}~\cite{wang2018cosface} &\multicolumn{1}{c}{21.7~/~21.7} & 72.9 & 74.3 & 83.0 & 90.2 & 82.6 & 79.5 \\
     ArcFace\textsuperscript{128}~\cite{deng2019arcface} &\multicolumn{1}{c}{21.7~/~21.7} & 62.3 & 20.4 & 57.7 & 49.1 & 53.2 & 38.8 \\
     CurricularFace\textsuperscript{128}~\cite{huang2020curricularface} &\multicolumn{1}{c}{21.7~/~21.7} & 76.9 & 77.5 & 82.7 & 89.4 & 83.0 & 81.3 \\
     Hyp\textsuperscript{128}~\cite{ermolov2022hyperbolic} &\multicolumn{1}{c}{21.7~/~21.7} &  75.5 & 56.8 & 83.7 & 90.3 & 81.7 & 74.2 \\
    \multicolumn{1}{l}{\ccol Ours\textsuperscript{128} }  & \multicolumn{1}{c}{\ccol \ccol 2.5~/~24.2} & \multicolumn{1}{c}{\ccol \textbf{82.5}} & \multicolumn{1}{c}{\ccol 84.6} &\multicolumn{1}{c}{ \ccol \textbf{84.9}}& \multicolumn{1}{c}{\ccol 91.5} & \multicolumn{1}{c}{\ccol \textbf{85.7}} & \ccol \textbf{85.7} \\      
\bottomrule
\end{tabularx}
\caption{Recall@1 of baselines and ours on the four standard benchmark datasets. Superscripts denote their embedding dimensions. We note that the result of ``Hyp'' presented in the table is obtained from our reimplementation.}
\label{subtab:comparison_standard}
\end{table*}
