# Supplementary material for: Learning Unified Distance Metric Across Diverse Data Distributions with Parameter-Efficient Transfer Learning
Source: arXiv:2309.08944 source file (2025-01-19)
Supplement: Supplementary file 6 [file backbone_ablation.tex]

\begin{table*}[!h]
\setlength{\tabcolsep}{2pt}
\fontsize{7.5}{9}\selectfont
\centering
\begin{tabularx}{1.0\textwidth}
    {
      p{0.05\textwidth}
      >{\centering\arraybackslash}p{0.14\textwidth}
      >{\centering\arraybackslash}X
      >{\centering\arraybackslash}X
      >{\centering\arraybackslash}X
      >{\centering\arraybackslash}X
      >{\centering\arraybackslash}X
      >{\centering\arraybackslash}X
      >{\centering\arraybackslash}X
      >{\centering\arraybackslash}X
      >{\centering\arraybackslash}X
      >{\centering\arraybackslash}X
      }
     \toprule

    \multicolumn{1}{l}{\multirow{2}{*}[-3.5mm]{Arch.}}&
    \multicolumn{1}{c}{\textbf{Params~(M)}} &
    \multicolumn{8}{c}{\textbf{Dataset-specific Accuracy}} & \multicolumn{2}{c}{\textbf{Universal Accuracy}} \\ 
    \cmidrule(lr){2-2}  \cmidrule(lr){3-10}  
    \cmidrule(lr){11-12} & 
    \multicolumn{1}{c}{Train~/~Total} &
    CUB & Cars & SOP & In\text{-}Shop & NABirds & Dogs & Flowers & Aircraft & Unified & Harmonic \\ \midrule
\multicolumn{1}{l}{ViT-S$^{128}$} & 2.5 / 24.2 & 83.9 & 84.3 & 84.0 & 89.8 & 79.2 & 84.1 & 99.3 & 72.6&  81.3 & 84.1 \\
\multicolumn{1}{l}{ViT-S$^{384}$} & 2.6 / 24.3 & 85.3 & 86.6 & 84.9 & 91.0 & 81.8 & 83.6 & 99.3 & 73.9&  82.8 & 85.3 \\
\multicolumn{1}{l}{ViT-B$^{128}$} & 5.0 / 90.8 & 85.7 & 88.2 & 86.0 & 92.2 & 83.0 & 87.5 & 99.4 & 78.8 & 84.0 & 87.2 \\
\multicolumn{1}{l}{ViT-L$^{128}$} & 12.9 / 316.2 & 86.6 & 88.7 & 86.9 & 93.2 & 84.4 & 90.8 & 99.4 & 78.5 & 84.8 & 88.2 \\
\multicolumn{1}{l}{ViT-L$^{128\dagger}$} & 6.6 / 309.9 & 86.8 & 90.5 & 86.3 & 92.8 & 85.3 & 90.9 & 99.3 & 79.5 & 84.9 & 88.6 \\
\bottomrule
\end{tabularx}
\caption{Recall@1 of PUMA using different backbones. 
The model denoted by $\dagger$ corresponds to a ViT-L architecture with adapters attached to the first 12 transformer layers, while the remaining models attach adapters to all transformer layers. The rest of the hyperparameters are the same.}
\label{subtab:backbone_ablation}
\end{table*}
