# Supplementary material for: Learning Unified Distance Metric Across Diverse Data Distributions with Parameter-Efficient Transfer Learning
Source: arXiv:2309.08944 source file (2025-01-19)
Supplement: Supplementary file 7 [file memory_ablation.tex]

\begin{table*}[!h]
\fontsize{7.5}{9}\selectfont
\centering
\begin{tabularx}{1.0\textwidth}
    {
      m{0.02\textwidth}
      >{\centering\arraybackslash}X
      >{\centering\arraybackslash}X
      >{\centering\arraybackslash}X
      >{\centering\arraybackslash}X
      >{\centering\arraybackslash}X
      >{\centering\arraybackslash}X
      >{\centering\arraybackslash}X
      >{\centering\arraybackslash}X
      >{\centering\arraybackslash}X
      >{\centering\arraybackslash}X
      >{\centering\arraybackslash}X
      >{\centering\arraybackslash}X}
     \toprule

    \multicolumn{1}{l}{\multirow{2}{*}[-3.5mm]{Methods}}&
    \multicolumn{8}{c}{\textbf{Dataset-specific Accuracy}} & \multicolumn{2}{c}{\textbf{Universal Accuracy}} \\ \cmidrule(lr){2-9}  
    \cmidrule(lr){10-11} & 
    CUB & Cars & SOP & InShop & NABirds & Dogs & Flowers & Aircraft & Unified & Harmonic \\ \midrule
\multicolumn{1}{l}{Triplet} & 75.2 & 36.5 & 78.5 & 79.9 & 69.3 & 78.3 & 98.7 & 39.8 & 71.1 & 62.3 \\
\multicolumn{1}{l}{MS} & 72.5 & 30.8 & 80.5 & 86.1 & 66.1 & 74.9 & 98.6 & 37.2 & 71.1 & 58.9 \\
\midrule
\multicolumn{1}{l}{Triplet + XBM} & 78.4 & 50.6 & 82.8 & 89.9 & 72.8 & 79.3 & 98.9 & 51.3 & 76.0 & 71.6 \\
\multicolumn{1}{l}{MS + XBM} & 78.1 & 55.1 & 84.3 & 91.5 & 72.4 & 79.6 & 98.0 & 54.7 & 77.0 & 73.7 \\
\bottomrule
\end{tabularx}
\caption{Comparison of the performance between pair-based losses with and without cross-batch memory.}
\label{subtab:memory_ablation}
\end{table*}
